# Supplementary material for: Work Statistics and Adiabatic Assumption in Nonequilibrium Many-Body Theory
Source: arXiv:2309.06258 source file (2023-09-21)
Supplement: Supplementary file 1 [file WSAA_SI.pdf]

# Supplementary Information for
# "Work Statistics and Adiabatic Assumption in Nonequilibrium Many-Body Theory"


Yi Zuo[1,6], Qinghong Yang[2,*] Bang-Gui Liu[1,6], and Dong E. Liu[2,3,4,5†]

[1] *Beijing National Laboratory for Condensed Matter Physics, and Institute of Physics, Chinese Academy of Sciences, Beijing 100190, China*

[2] *State Key Laboratory of Low Dimensional Quantum Physics, Department of Physics, Tsinghua University, Beijing, 100084, China*

[3] *Beijing Academy of Quantum Information Sciences, Beijing 100193, China*

[4] *Frontier Science Center for Quantum Information, Beijing 100184, China*

[5] *Hefei National Laboratory, Hefei 230088, China and*

[6] *University of Chinese Academy of Science, Beijing 100046, China*


In this supplementary information,we provide detailed proofs of lemmas and the theorem given in the main text in Sec. I, show how to calculate the third order cumulant CFW (characteristic function of work) and discuss the property of cumulant correlation functions in Sec. II.

## I. PROOFS OF LEMMAS AND THE THEOREM

In the following, we show proofs of lemmas and the theorem given in the main text. For convenience, we also rewrite those lemmas and the theorem here.

**Lemma 1.** The averaged work $\langle w\rangle \equiv \int dwwp\left(w\right)$ of an evolution from $t_i$ to $t_f$, can also be expressed as $\langle w\rangle = \langle H\left(t_f\right)\rangle_{t_f} - \langle H\left(t_i\right)\rangle_{t_i}$, where $\langle H\left(t\right)\rangle_t \equiv \mathrm{tr}\left[\rho\left(t\right)H\left(t\right)\right]$.

**Proof.** This can be easily proved from the definition of the work distribution $p(w)$.

Note that

$$p\left(w\right) = \sum_{n,m}\delta\left[w-\left(E_m^f-E_n^i\right)\right]\left|\langle\psi_m^f\left|U\left(t_f\right)\right|\psi_n^i\rangle\right|^2\frac{e^{-\beta E_n^i}}{Z\left(t_i\right)}, \tag{1}$$

thus the averaged work for all trajectories is given by

$$\begin{aligned}
\langle w\rangle &= \int dww\sum_{n,m}\delta\left[w-\left(E_m^f-E_n^i\right)\right]\left|\langle E_m^f|U\left(t_f\right)|E_n^i\rangle\right|^2\frac{e^{-\beta E_n^i}}{Z\left(t_i\right)}\\
&= \sum_{n,m}\left|\langle E_m^f|U\left(t_f\right)|E_n^i\rangle\right|^2\frac{e^{-\beta E_n^i}}{Z\left(t_i\right)}\left(E_m^f-E_n^i\right)\\
&= \sum_{n,m}\langle E_n^i|U^\dagger\left(t_f\right)|E_m^f\rangle\langle E_m^f|U\left(t_f\right)|E_n^i\rangle\frac{e^{-\beta E_n^i}}{Z\left(t_i\right)}E_m^f\\
&\quad-\sum_{n,m}\langle E_n^i|U^\dagger\left(t_f\right)|E_m^f\rangle\langle E_m^f|U\left(t_f\right)|E_n^i\rangle\frac{e^{-\beta E_n^i}}{Z\left(t_i\right)}E_n^i\\
&= \sum_{n}\langle E_n^i|U^\dagger\left(t_f\right)\sum_m E_m^f|E_m^f\rangle\langle E_m^f|U\left(t_f\right)\frac{e^{-\beta E_n^i}}{Z\left(t_i\right)}|E_n^i\rangle\\
&\quad-\sum_{n}\langle E_n^i|U^\dagger\left(t_f\right)\sum_m|E_m^f\rangle\langle E_m^f|U\left(t_f\right)|E_n^i\rangle\frac{e^{-\beta E_n^i}}{Z\left(t_i\right)}E_n^i\\
&= \mathrm{tr}\left[U^\dagger\left(t_f\right)H\left(t_f\right)U\left(t_f\right)\rho\left(t_i\right)\right]-\mathrm{tr}\left[H\left(t_i\right)\rho\left(t_i\right)\right]\\
&= \mathrm{tr}\left[H\left(t_f\right)\rho\left(t_f\right)\right]-\mathrm{tr}\left[H\left(t_i\right)\rho\left(t_i\right)\right]\\
&\equiv \langle H\left(t_f\right)\rangle_{t_f}-\langle H\left(t_i\right)\rangle_{t_i}.
\end{aligned} \tag{2}$$


* yqh19@mails.tsinghua.edu.cn

† dongeliu@mail.tsinghua.edu.cn

□

**Lemma 2.** Suppose there exists an evolution protocol from $t_i$ to $t_f$, such that for all systems, the average work of the evolution satisfies $\langle w\rangle = \langle H(t_f)\rangle_G - \langle H(t_i)\rangle_{t_i}$, where

$$\langle H(t_f)\rangle_G \equiv \frac{1}{\mathrm{tr}\left[e^{-\beta H(t_f)}\right]}\,\mathrm{tr}\left[e^{-\beta H(t_f)}H(t_f)\right],$$

then the final state $\rho(t_f)$ is a Gibbs state with respect to $H(t_f)$ at inverse temperature $\beta$.

**Proof.** From Lemma 1, one has $\langle w\rangle = \langle H(t_f)\rangle_{t_f} - \langle H(t_i)\rangle_{t_i}$. If for all systems, an evolution makes $\langle w\rangle = \langle H(t_f)\rangle_G - \langle H(t_i)\rangle_{t_i}$, then one has $\langle H(t_f)\rangle_G = \langle H(t_f)\rangle_{t_f}$, which leads to

$$\begin{aligned}\frac{1}{\mathrm{tr}\left[e^{-\beta H(t_f)}\right]}\,\mathrm{tr}\left[e^{-\beta H(t_f)}H(t_f)\right] &= \mathrm{tr}\left[H(t_f)\,\rho(t_f)\right]\\ \mathrm{tr}\left\{H(t_f)\left[\rho(t_f) - \frac{1}{\mathrm{tr}\left[e^{-\beta H(t_f)}\right]}e^{-\beta H(t_f)}\right]\right\} &= 0.\end{aligned} \tag{3}$$

Since the above equation holds for arbitrary $H(t_f)$ (all systems), $\rho(t_f)$ should satisfy

$$\rho(t_f) = \frac{1}{\mathrm{tr}\left[e^{-\beta H(t_f)}\right]}e^{-\beta H(t_f)}, \tag{4}$$

that is the final state should be a Gibbs state with respect to $H(t_f)$ at inverse temperature $\beta$.

□

Having proved the above two lemmas, one can use them to prove the Theorem 1 given in the main text.

**Theorem 1.** Suppose there exists an evolution protocol from $t_i$ to $t_f$, such that for *all* systems, the evolution will drive the initial Gibbs state $\rho(t_i) = e^{-\beta H(t_i)}/Z(t_i)$ to a final state (at $t_f$), which is a Gibbs state with respect to $H(t_f)$ at inverse termperature $\beta$. This evolution protocol exists *if and only if* the work distribution $p(w)$ is a delta function for all systems.

**Proof. a**). We first prove the sufficiency: If the work distribution is $p(w) = \delta(w - w_0)$ (For different systems, $w_0$ can be different), then the work of each trajectory should be the same, and equals to the average $\langle w\rangle$. According to the Jarzynski equality Eq. (8), one has

$$\langle e^{-\beta w}\rangle = e^{-\beta w_0} = \frac{Z(t_f)}{Z(t_i)}, \tag{5}$$

where $Z(t_f)$ is the partition function of a *hypothetical* system with Hamiltonian $H(t_f)$ in a Gibbs state at inverse temperature $\beta$. Then

$$\begin{aligned} w_0 &= -\frac{\partial}{\partial\beta}\ln\frac{Z(t_f)}{Z(t_i)}\\ \Rightarrow \langle w\rangle &= -\frac{\partial}{\partial\beta}\ln\frac{Z(t_f)}{Z(t_i)}\\ &= -\frac{\partial \ln Z(t_f)}{\partial\beta} + \frac{\partial \ln Z(t_i)}{\partial\beta}\\ &= \frac{1}{\mathrm{tr}\left[e^{-\beta H(t_f)}\right]}\,\mathrm{tr}\left[H(t_f)\,e^{-\beta H(t_f)}\right] - \mathrm{tr}\left[H(t_i)\,\rho(t_i)\right]\\ &\equiv \langle H(t_f)\rangle_G - \langle H(t_i)\rangle_{t_i}.\end{aligned} \tag{6}$$

According to Lemma 2, we know that the state of the *real* system at $t_f$ is also the Gibbs state $\rho(t_f) = \exp\left[-\beta H(t_f)\right]/Z(t_f)$.

**b**). We then prove the necessity: If the state at $t_f$ is $\rho(t_f) = \exp\left[-\beta H(t_f)\right]/Z(t_f)$, then according to Lemma 1, one has

$$\begin{aligned}\langle w\rangle &= \langle H(t_f)\rangle_{t_f} - \langle H(t_i)\rangle_{t_i}\\ &= \mathrm{tr}\left[H(t_f)\,\rho(t_f)\right] - \mathrm{tr}\left[H(t_i)\,\rho(t_i)\right]\\ &= -\frac{\partial \ln Z(t_f)}{\partial\beta} + \frac{\partial \ln Z(t_i)}{\partial\beta}\\ &= -\frac{\partial}{\partial\beta}\ln\frac{Z(t_f)}{Z(t_i)}.\end{aligned} \tag{7}$$

In addition, the Jarzynski equality gives

$$\begin{aligned} \langle e^{-\beta w}\rangle &= \frac{Z\left(t_f\right)}{Z\left(t_i\right)} \\ \Rightarrow -\frac{\partial}{\partial\beta}\ln\langle e^{-\beta w}\rangle &= -\frac{\partial}{\partial\beta}\ln\frac{Z\left(t_f\right)}{Z\left(t_i\right)}. \end{aligned} \tag{8}$$

Combinging Eq. (7) and Eq. (8), one has

$$\begin{aligned} \langle w\rangle &= -\frac{\partial}{\partial\beta}\ln\langle e^{-\beta w}\rangle \\ \Rightarrow \langle w\rangle &= \frac{1}{\langle e^{-\beta w}\rangle}\langle w e^{-\beta w}\rangle \\ \Rightarrow \quad 0 &= \langle w\left(\frac{1}{\langle e^{-\beta w}\rangle}e^{-\beta w}-1\right)\rangle. \end{aligned} \tag{9}$$

Since this equation holds for *all* systems, the outer $\langle\cdot\rangle$ operation can be dropped, that is

$$\begin{aligned} 0 &= \frac{1}{\langle e^{-\beta w}\rangle}e^{-\beta w}-1 \\ \Rightarrow e^{-\beta w} &= \langle e^{-\beta w}\rangle \\ \Rightarrow \quad w &= w_0, \end{aligned} \tag{10}$$

where $w_0$ is a constant but can be different for different systems. Therefore, the work distribution for the desired evolution protocol should be

$$p(w) = \delta(w-w_0). \tag{11}$$

Since $w_0$ corresponds to work, it should be a real number.

□

Expressing Theorem 1 through the characteristic function of work leads to the following corollary:

**Corollary 1.** The logarithm of the characteristic function of work $\chi(u)$ for the evolution protocol given by Theorem 1 satisfies $\ln\chi(u) = iuw_0$, where $w_0$ is a real number.

**Proof.** This can be directly obtained from the Fourier transformation of $p(w) = \delta(w-w_0)$:

$$\begin{aligned} \ln\chi(u) &= \ln\left[\int dw p(w)e^{iuw}\right] \\ &= \ln\left[\int dw\delta(w-w_0)e^{iuw}\right] \\ &= \ln e^{iuw_0} \\ &= iuw_0. \end{aligned} \tag{12}$$

□

## II. CALCULATIONS OF CUMULANT CFW

For general evolution protocols, the logarithmic CFW is calculated up to $\mathcal{O}(\lambda_1^2)$ in Ref. [1]. Using parameters defined in our work, it can be expressed as

$$\ln\chi\left(u\right) = iu\lambda_1\langle H_1\rangle_c + iu\lambda_1^2\int_{-\infty}^{\infty}\frac{d\omega}{2\pi}\frac{G_c^{>}(\omega)}{\omega} + \int_{-\infty}^{\infty}\frac{d\omega}{2\pi}\frac{1-e^{i\omega u}}{\omega^2}A(\omega)G_c^{>}(\omega) + \mathcal{O}(\lambda_1^3), \tag{13}$$

where $A(\omega) \equiv |\int_0^t ds\dot{\lambda}(s)e^{i\omega s}|^2$. The first two terms are linear $u$. As our theorem or corollary requires that the $\chi(u)$ of the desired NI protocol should satisfy $\ln\chi(u) = iuw_0$ with $w_0$ being a real number, in order to see whether the

second term matches our theorem, we need to know that is $G_c^>(\omega)$ a real function. Note that

$$\begin{aligned}
&G_c\left(s_1,s_2\right)\\
=&-\langle H_1^I\left(s_1\right)H_1^I\left(s_2\right)\rangle_c\\
=&-\langle H_1^I\left(s_1\right)H_1^I\left(s_2\right)\rangle_0+\langle H_1^I\left(s_1\right)\rangle\langle H_1^I\left(s_2\right)\rangle_0\\
=&-\langle H_1^I\left(s_1\right)H_1^I\left(s_2\right)\rangle_0+\langle H_1\rangle\langle H_1\rangle_0\\
=&-\frac{1}{\mathrm{tr}\left(e^{-\beta H_0}\right)}\mathrm{tr}\left[e^{-\beta H_0}H_1^I\left(s_1\right)H_1^I\left(s_2\right)\right]+\langle H_1\rangle_0\langle H_1\rangle_0\\
=&-\frac{1}{\mathrm{tr}\left(e^{-\beta H_0}\right)}\mathrm{tr}\left[e^{-\beta H_0}e^{iH_0s_1}H_1e^{-iH_0s_1}e^{iH_0s_2}H_1e^{-iH_0s_2}\right]+\langle H_1\rangle_0\langle H_1\rangle_0\\
=&-\frac{1}{\mathrm{tr}\left(e^{-\beta H_0}\right)}\mathrm{tr}\left[e^{-\beta H_0}e^{iH_0(s_1-s_2)}H_1e^{-iH_0(s_1-s_2)}H_1\right]+\langle H_1\rangle_0\langle H_1\rangle_0\\
\equiv&-\langle H_1^I\left(s_1-s_2\right)H_1^I\left(0\right)\rangle_0+\langle H_1\rangle_0\langle H_1\rangle_0\\
\equiv&G_c^>\left(s_1-s_2\right),
\end{aligned}\tag{14}$$

thus one has

$$\left[G_c^>\left(s_1-s_2\right)\right]^*=G_c^>\left(s_2-s_1\right).\tag{15}$$

Therefore,

$$\begin{aligned}
[G_c^>(\omega)]^*&=\int_{-\infty}^{+\infty}ds[G_c^>(s)]^*e^{-i\omega s}\\
&=\int_{-\infty}^{+\infty}ds[G_c^>(-s)]^*e^{i\omega s}\\
&=\int_{-\infty}^{+\infty}dsG_c^>(s)e^{i\omega s}\\
&=G_c^>(\omega),
\end{aligned}\tag{16}$$

which means $G_c^>(\omega)$ is a real function, and thus $\lambda_1^2\int_{-\infty}^{+\infty}\frac{d\omega}{2\pi}\frac{G_c^>(\omega)}{\omega}$ in the second term of Eq. (13) is a real number. Therefore, the first two terms in Eq. (13) matches our theorem.

For non-adiabatic evolution protocols, $\dot{\lambda}(s)\neq 0$, thus $A(\omega)\neq 0$. Thus, for non-adiabatic evolutions, $\ln\chi(u)$ is already nonlinear in $u$ when we keep terms up to the second order of $\lambda_1$. Therefore, the logarithmic CFW of non-adiabatic evolutions deviates from our theorem (or the corollary) up to $\mathcal{O}(\lambda_1^2)$. However, for adiabatic cases, $t\to\infty$ and $\dot{\lambda}(s)\to 0$, thus the third term containing $A(\omega)$ in Eq. (13) approaches to 0. That is to say, for adiabatic evolutions, the logarithmic CFW $\ln\chi(u)$ is linear in $u$ when we keep terms up to $\mathcal{O}(\lambda_1^2)$, and thus matches our theorem (or corollary) up to $\mathcal{O}(\lambda_1^2)$. So the question is will $\ln\chi(u)$ of adiabatic evolutions matches our theorem for all orders? To answer this question, we calculate the third order of $\ln\chi(u)$:

$$\begin{aligned}
&\int_C d\bar{s}_1\int_C d\bar{s}_2\int_C d\bar{s}_3G_c\left(s_1,s_2,s_3\right)\\
=&\int_C d\bar{s}_1\int_C d\bar{s}_2\int_C d\bar{s}_3G_c^>\left(s_1-s_3,s_2-s_3\right)\\
=&\int_{-\infty}^{\infty}\int_{-\infty}^{\infty}\frac{d\omega_1}{2\pi}\frac{d\omega_2}{2\pi}G_c^>\left(\omega_1,\omega_2\right)\int_C d\bar{s}_1\int_C d\bar{s}_2\int_C d\bar{s}_3e^{-i\omega_1(s_1-s_3)}e^{-i\omega_2(s_2-s_3)},
\end{aligned}\tag{17}$$

where $C$ is the time contour for work statistics provided in the main text, and $d\bar{s}_l\equiv ds_l\lambda_C(s)\theta_C(s_l-s_{l+1})$ with $\theta_C(s_l-s_{l+1})$ being the contour step function. $\lambda_C(s)$ is a piecewise function along $C$, and is defined as:

- Part 1: $s\in[0,t]$, $\lambda_C(s)=\lambda_(s)$;
- Part 2: $s\in[t,t-u]$, $\lambda_C(s)=\lambda_1$;
- Part 3: $s\in[t-u,-u]$, $\lambda_C(s)=\lambda(s+u)$;

- Part 4: $s \in [-u, 0]$, $\lambda_C(s) = \lambda_0 = 0$.

Thus, $\int_C d\bar{s}_1 \int_C d\bar{s}_2 \int_C d\bar{s}_3$ can be divided into 64 terms, which will be labeled by $(i, j, k)$. However, due to the order in the contour and $\lambda_0 = 0$, only 10 terms remain, and they are

$$(i, j, k) = (1, 1, 1), (2, 1, 1), (2, 2, 1), (2, 2, 2), (3, 1, 1), (3, 2, 1), (3, 2, 2), (3, 3, 1), (3, 3, 2), (3, 3, 3). \tag{18}$$

In the following, we show calculations of $(2, 1, 1)$ and $(3, 1, 1)$, and directly gives the results of other terms. For adiabatic case, we will set $t \to \infty$ and $\dot{\lambda}(s) \to 0$, while keep $\dot{\lambda}(s)t$ finite.

For $(i, j, k) = (2, 1, 1)$, one has

$$\begin{aligned}
&\int_t^{t-u} d\bar{s}_1 \int_0^t d\bar{s}_2 \int_0^t d\bar{s}_3 e^{-i\omega_1 s_1} e^{-i\omega_2 s_2} e^{i(\omega_1+\omega_2)s_3} \\
=&\int_t^{t-u} ds_1 \int_0^t ds_2 \int_0^{s_2} ds_3 e^{-i\omega_1 s_1} e^{-i\omega_2 s_2} e^{i(\omega_1+\omega_2)s_3} \lambda_1 \lambda(s_2) \lambda(s_3) \\
=&\int_t^{t-u} ds_1 \int_0^t ds_2 e^{-i\omega_1 s_1} e^{-i\omega_2 s_2} \lambda_1 \lambda(s_2) \int_0^{s_2} ds_3 e^{i(\omega_1+\omega_2)s_3} \lambda(s_3) \\
=&\int_t^{t-u} ds_1 \int_0^t ds_2 e^{-i\omega_1 s_1} e^{-i\omega_2 s_2} \lambda_1 \lambda(s_2) \left[ \frac{\lambda(s_3) e^{i(\omega_1+\omega_2)s_3}}{i(\omega_1+\omega_2)} \Bigg|_0^{s_2} - \int_0^{s_2} ds_3 \frac{\dot{\lambda}(s_3) e^{i(\omega_1+\omega_2)s_3}}{i(\omega_1+\omega_2)} \right] \\
=&\int_t^{t-u} ds_1 \int_0^t ds_2 e^{-i\omega_1 s_1} e^{-i\omega_2 s_2} \lambda_1 \lambda(s_2) \frac{\lambda(s_2) e^{i(\omega_1+\omega_2)s_2}}{i(\omega_1+\omega_2)} \\
=&\int_t^{t-u} ds_1 e^{-i\omega_1 s_1} \lambda_1 \int_0^t ds_2 \frac{\lambda^2(s_2) e^{i\omega_1 s_2}}{i(\omega_1+\omega_2)} \\
=&\int_t^{t-u} ds_1 e^{-i\omega_1 s_1} \lambda_1 \left[ \frac{\lambda^2(s_2) e^{i\omega_1 s_2}}{-\omega_1(\omega_1+\omega_2)} \Bigg|_0^t - \int_0^t ds_2 \frac{2\lambda(s_2)\dot{\lambda}(s_2) e^{i\omega_1 s_2}}{-\omega_1(\omega_1+\omega_2)} \right] \\
=&\int_t^{t-u} ds_1 e^{-i\omega_1 s_1} \lambda_1 \frac{\lambda^2(t) e^{i\omega_1 t}}{-\omega_1(\omega_1+\omega_2)} \\
=&\frac{\lambda_1^3 e^{i\omega_1 t}}{-\omega_1(\omega_1+\omega_2)} \int_t^{t-u} ds_1 e^{-i\omega_1 s_1} \\
=&\frac{\lambda_1^3 \left(e^{i\omega_1 u} - 1\right)}{i\omega_1^2(\omega_1+\omega_2)},
\end{aligned} \tag{19}$$

For $(i, j, k) = (3, 1, 1)$, one has

$$\begin{aligned}
&\int_{t-u}^{-u} d\bar{s}_1 \int_0^t d\bar{s}_2 \int_0^t d\bar{s}_3 e^{-i\omega_1 s_1} e^{-i\omega_2 s_2} e^{i(\omega_1+\omega_2)s_3} \\
=&\int_t^0 ds_1 \int_0^t ds_2 \int_0^{s_2} ds_3 e^{-i\omega_1 s_1} e^{-i\omega_2 s_2} e^{i(\omega_1+\omega_2)s_3} \lambda(s_1) \lambda(s_2) \lambda(s_3) e^{i\omega_1 u} \\
=&\int_t^0 ds_1 \int_0^t ds_2 e^{-i\omega_1 s_1} e^{-i\omega_2 s_2} \lambda(s_1) \lambda(s_2) \int_0^{s_2} ds_3 e^{i(\omega_1+\omega_2)s_3} \lambda(s_3) e^{i\omega_1 u} \\
=&\int_t^0 ds_1 e^{i\omega_1 u} e^{-i\omega_1 s_1} \lambda(s_1) \int_0^t ds_2 \lambda(s_2) \frac{\lambda(s_2) e^{i\omega_1 s_2}}{i(\omega_1+\omega_2)} \\
=&e^{i\omega_1 u} \int_t^0 ds_1 e^{-i\omega_1 s_1} \lambda(s_1) \frac{\lambda^2(t) e^{i\omega_1 t}}{-\omega_1(\omega_1+\omega_2)} \\
=&e^{i\omega_1 u} \frac{\lambda^2(t) e^{i\omega_1 t}}{-\omega_1(\omega_1+\omega_2)} \frac{\lambda(t) e^{-i\omega_1 t}}{i\omega_1} \\
=&\frac{\lambda_1^3 e^{i\omega_1 u}}{-i\omega_1^2(\omega_1+\omega_2)}.
\end{aligned} \tag{20}$$

We now provide results of other terms:

$$(1, 1, 1) = \frac{1}{-\omega_1(\omega_1+\omega_2)} \lambda_1^3 t. \tag{21}$$

$$(2,2,1) = \frac{i\lambda_1^3}{\omega_2\left(\omega_1+\omega_2\right)}\left[\frac{e^{i(\omega_1+\omega_2)u}-1}{\left(\omega_1+\omega_2\right)} - \frac{e^{i\omega_1 u}-1}{\omega_1}\right]. \tag{22}$$

$$(2,2,2) = \lambda_1^3\left[\frac{i\omega_1 u - e^{i\omega_1 u}+1}{i\omega_1^2\left(\omega_1+\omega_2\right)} - \frac{e^{i(\omega_1+\omega_2)u}-1}{-i\omega_2\left(\omega_1+\omega_2\right)^2} + \frac{e^{i\omega_1 u}-1}{-i\omega_1\omega_2\left(\omega_1+\omega_2\right)}\right]. \tag{23}$$

$$(3,1,1) = \frac{\lambda_1^3 e^{i\omega_1 u}}{-i\omega_1^2\left(\omega_1+\omega_2\right)}. \tag{24}$$

$$(3,2,1) = \frac{\lambda_1^3 e^{i\omega_1 u}\left(e^{i\omega_2 u}-1\right)}{i\omega_1\omega_2\left(\omega_1+\omega_2\right)}. \tag{25}$$

$$(3,2,2) = \frac{\lambda_1^3}{-\omega_1\left(\omega_1+\omega_2\right)}\left[\frac{1-e^{i\omega_1 u}}{i\omega_1} + \frac{e^{i(\omega_1+\omega_2)u}-e^{i\omega_1 u}}{i\omega_2}\right]. \tag{26}$$

$$(3,3,1) = -\frac{\lambda_1^3}{i\omega_1\left(\omega_1+\omega_2\right)^2}e^{i(\omega_1+\omega_2)u}. \tag{27}$$

$$(3,3,2) = \lambda_1^3\frac{\left(1-e^{i(\omega_1+\omega_2)u}\right)}{\omega_2\left(\omega_1+\omega_2\right)}\left[\frac{1}{i(\omega_1+\omega_2)} - \frac{1}{i\omega_1}\right]. \tag{28}$$

$$(3,3,3) = \frac{\lambda_1^3 t}{\omega_1\left(\omega_1+\omega_2\right)} + \frac{\lambda_1^3}{i\left(\omega_1+\omega_2\right)\omega_1^2} - \frac{\lambda_1^3}{i\left(\omega_1+\omega_2\right)^2\omega_2} + \frac{\lambda_1^3}{i\left(\omega_1+\omega_2\right)\omega_1\omega_2}. \tag{29}$$

Sum those ten terms up, one gets

$$\begin{aligned}&\int_{-\infty}^{\infty}\int_{-\infty}^{\infty}\frac{d\omega_1}{2\pi}\frac{d\omega_2}{2\pi}G_c^{>}(\omega_1,\omega_2)\int_C d\bar{s}_1\int_C d\bar{s}_2\int_C d\bar{s}_3 e^{-i\omega_1(s_1-s_3)}e^{-i\omega_2(s_2-s_3)}\\ =\, & iu\lambda_1^3\int_{-\infty}^{\infty}\int_{-\infty}^{\infty}\frac{d\omega_1}{2\pi}\frac{d\omega_2}{2\pi}\frac{G_c^{>}(\omega_1,\omega_2)}{i\omega_1(\omega_1+\omega_2)}.\end{aligned} \tag{30}$$

At the first glance, one may think that the third order term is also linear in $u$, and thus also matches our theorem (or corollary). However, our theorem (corollary) requires that $\ln\chi(u) = iuw_0$ with $w_0$ being a real number for the desired evolution protocol. Therefore, we still need to know the property of $G_c^{>}(\omega_1,\omega_2)$. Similar with procedures in demonstrating that $G_c^{>}(\omega)$ is a real function, one can prove that $G_c^{>}(\omega_1,\omega_2)$ is a complex function. Note that

$$\begin{aligned}&G_c(s_1,s_2,s_3)\\ =&G_c^{>}(s_1-s_3,s_2-s_3)\\ \equiv&(-i)^3\langle H_1^I(s_1-s_3)\,H_1^I(s_2-s_3)\,H_1^I(0)\rangle_c\\ =&i\left\{\langle H_1^I(s_1-s_3)\,H_1^I(s_2-s_3)\,H_1^I(0)\rangle_0\right.\\ &-\left[\langle H_1^I(s_1-s_3)\rangle_0\langle H_1^I(s_2-s_3)\,H_1^I(0)\rangle_0+\langle H_1^I(s_2-s_3)\rangle_0\langle H_1^I(0)\,H_1^I(s_1-s_3)\rangle_0+\langle H_1^I(0)\rangle_0\langle H_1^I(s_1-s_3)\,H_1^I(s_2-s_3)\rangle_0\right]\\ &\left.+2\langle H_1^I(s_1-s_3)\rangle_0\langle H_1^I(s_2-s_3)\rangle_0\langle H_1^I(0)\rangle_0\right\}.\end{aligned} \tag{31}$$

According to Eqs. (14) and (15), Fourier transformations of the last two lines of Eq. (31) are all real. Therefore, in order to check whether $G_c^{>}(\omega_1,\omega_2)$ is a complex function, we just need to focus on $\langle H_1^I(s_1-s_3)\,H_1^I(s_2-s_3)\,H_1^I(0)\rangle$.

For convenience, we let $G_c^>(s_1-s_2,s_2-s_3)\equiv i\underline{G}_c^>(s_1-s_2,s_2-s_3)$. Then, we have

$$\begin{aligned}
&\underline{G}(s_1-s_3,s_2-s_3)\\
\equiv&\langle H_1^I(s_1-s_3)H_1^I(s_2-s_3)H_1^I(0)\rangle_0\\
=&\frac{1}{\operatorname{tr}(e^{-\beta H_0})}\operatorname{tr}\left[e^{-\beta H_0}H_1^I(s_1-s_3)H_1^I(s_2-s_3)H_1^I(0)\right]\\
=&\frac{1}{\operatorname{tr}(e^{-\beta H_0})}\operatorname{tr}\left[e^{-\beta H_0}e^{iH_0(s_1-s_3)}H_1e^{-iH_0(s_1-s_3)}e^{iH_0(s_2-s_3)}H_1e^{-iH_0(s_2-s_3)}H_1\right],
\end{aligned}\tag{32}$$

and

$$\begin{aligned}
&[\underline{G}(s_1-s_3,s_2-s_3)]^*\\
=&\frac{1}{\operatorname{tr}(e^{-\beta H_0})}\operatorname{tr}\left[H_1e^{iH_0(s_2-s_3)}H_1e^{-iH_0(s_2-s_3)}e^{iH_0(s_1-s_3)}H_1e^{-iH_0(s_1-s_3)}e^{-\beta H_0}\right]\\
=&\frac{1}{\operatorname{tr}(e^{-\beta H_0})}\operatorname{tr}\left[e^{-\beta H_0}H_1e^{iH_0(s_2-s_3)}H_1e^{-iH_0(s_2-s_3)}e^{iH_0(s_1-s_3)}H_1e^{-iH_0(s_1-s_3)}\right]\\
=&\frac{1}{\operatorname{tr}(e^{-\beta H_0})}\operatorname{tr}\left[e^{-\beta H_0}e^{-iH_0(s_1-s_3)}H_1e^{iH_0(s_2-s_3)}e^{-iH_0(s_2-s_1)}e^{iH_0(s_2-s_1)}H_1e^{-iH_0(s_2-s_1)}H_1\right]\\
=&\frac{1}{\operatorname{tr}(e^{-\beta H_0})}\operatorname{tr}\left[e^{-\beta H_0}e^{-iH_0(s_1-s_3)}H_1e^{iH_0(s_1-s_3)}e^{iH_0(s_2-s_1)}H_1e^{-iH_0(s_2-s_1)}H_1\right]\\
=&\langle H_1^I(s_3-s_1)H_1^I(s_2-s_1)H_1^I(0)\rangle_0\\
\equiv&\underline{G}(s_3-s_1,s_2-s_1).
\end{aligned}\tag{33}$$

Note that

$$\begin{aligned}
&\underline{G}(s_3-s_1,s_3-s_2)-\underline{G}(s_3-s_1,s_2-s_1)\\
=&\frac{1}{\operatorname{tr}(e^{-\beta H_0})}\operatorname{tr}\left[e^{-\beta H_0}e^{iH_0(s_3-s_1)}H_1e^{-iH_0(s_3-s_1)}e^{iH_0(s_3-s_2)}H_1e^{-iH_0(s_3-s_2)}H_1\right]\\
&-\frac{1}{\operatorname{tr}(e^{-\beta H_0})}\operatorname{tr}\left[e^{-\beta H_0}e^{iH_0(s_3-s_1)}H_1e^{-iH_0(s_3-s_1)}e^{iH_0(s_2-s_1)}H_1e^{-iH_0(s_2-s_1)}H_1\right]\\
=&\frac{1}{\operatorname{tr}(e^{-\beta H_0})}\operatorname{tr}\left[e^{-\beta H_0}e^{iH_0(s_3-s_1)}H_1e^{-iH_0(s_3-s_1)}\left\{e^{iH_0(s_3-s_2)}H_1e^{-iH_0(s_3-s_2)}-e^{iH_0(s_2-s_1)}H_1e^{-iH_0(s_2-s_1)}\right\}H_1\right],
\end{aligned}\tag{34}$$

thus, if $[H_0,H_1]\neq0$ which always holds for interacting systems, one has $\underline{G}(s_3-s_1,s_3-s_2)\neq\underline{G}(s_3-s_1,s_2-s_1)=[\underline{G}(s_1-s_3,s_2-s_3)]^*$. Therefore, one has

$$\begin{aligned}
\left[\underline{G}_c^>(\omega_1,\omega_2)\right]^*&=\int_{-\infty}^{+\infty}ds\int_{-\infty}^{+\infty}ds'\left[\underline{G}_c^>(s,s')\right]^*e^{-i\omega_1s}e^{-i\omega_2s'}\\
&=\int_{-\infty}^{+\infty}ds\int_{-\infty}^{+\infty}ds'\left[\underline{G}_c^>(-s,-s')\right]^*e^{i\omega_1s}e^{i\omega_2s'}\\
&\neq\int_{-\infty}^{+\infty}ds\int_{-\infty}^{+\infty}ds'\underline{G}_c^>(s,s')e^{i\omega_1s}e^{i\omega_2s'}\\
&=\underline{G}_c^>(\omega_1,\omega_2),
\end{aligned}\tag{35}$$

which means $\underline{G}_c^>(\omega_1,\omega_2)$ is a complex function instead of a real function. Thus, $G_c^>(\omega_1,\omega_2)$ is not purely imaginary, and $\int_{-\infty}^{\infty}\int_{-\infty}^{\infty}\frac{d\omega_1}{2\pi}\frac{d\omega_2}{2\pi}\frac{G_c^>(\omega_1,\omega_2)}{i\omega_1(\omega_1+\omega_2)}$ will not be a real number. Therefore, the third order of $\ln\chi(u)$, Eq. (30) in the adiabatic case does not match our theorem. That is to say, $\ln\chi(u)$ of the adiabatic evolution protocol deviates from our theorem (or corollary) when we keep terms up to $\mathcal{O}(\lambda_1^3)$.

---

[1] Z. Fei and H. T. Quan, Phys. Rev. Lett. **124**, 240603 (2020).
